# Supplementary material for: ICMarks: A Robust Watermarking Framework for Integrated Circuit Physical Design IP Protection
Source: arXiv:2404.18407 source file (2025-03-12)
Supplement: Supplementary file 1 [file appendix.tex]

\clearpage

\onecolumn

\section*{Appendix}


 
\subsection{Additional Watermarked Design Example}\label{sec:addition_exp}

We include the additional watermarked design visualization in this subsection. 



\begin{figure*}[!ht]
    \centering
    \subfloat[fft\_a (WM)]{\label{subf:design1} \includegraphics[width=0.2\linewidth]{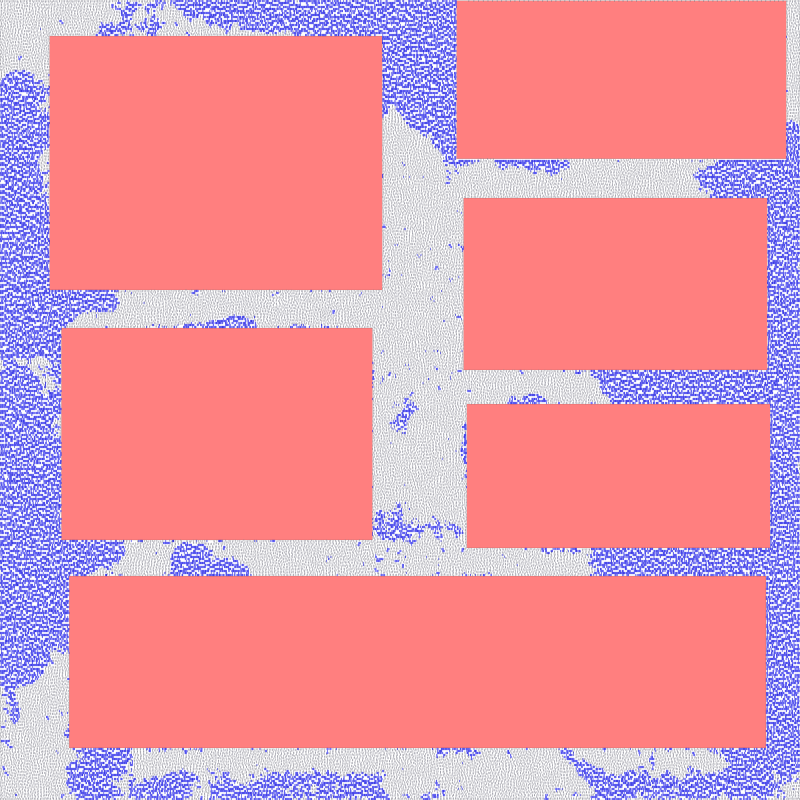}}
    \subfloat[fft\_a (non-WM)]{\label{subf:design1} \includegraphics[width=0.2\linewidth]{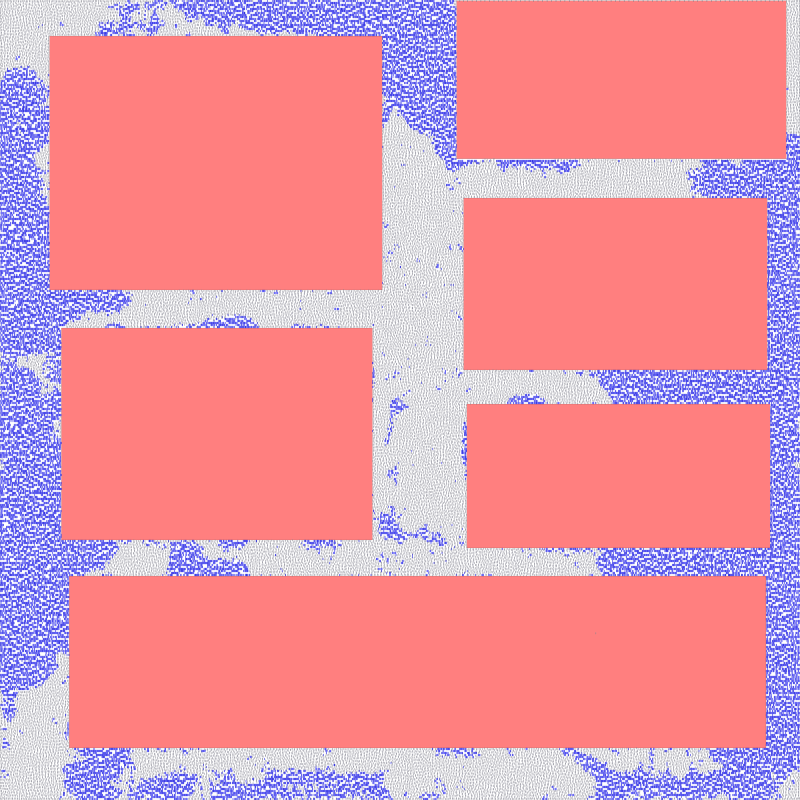}}
    \subfloat[pci\_a (WM)]{\label{f:design3} \includegraphics[width=0.2\linewidth]{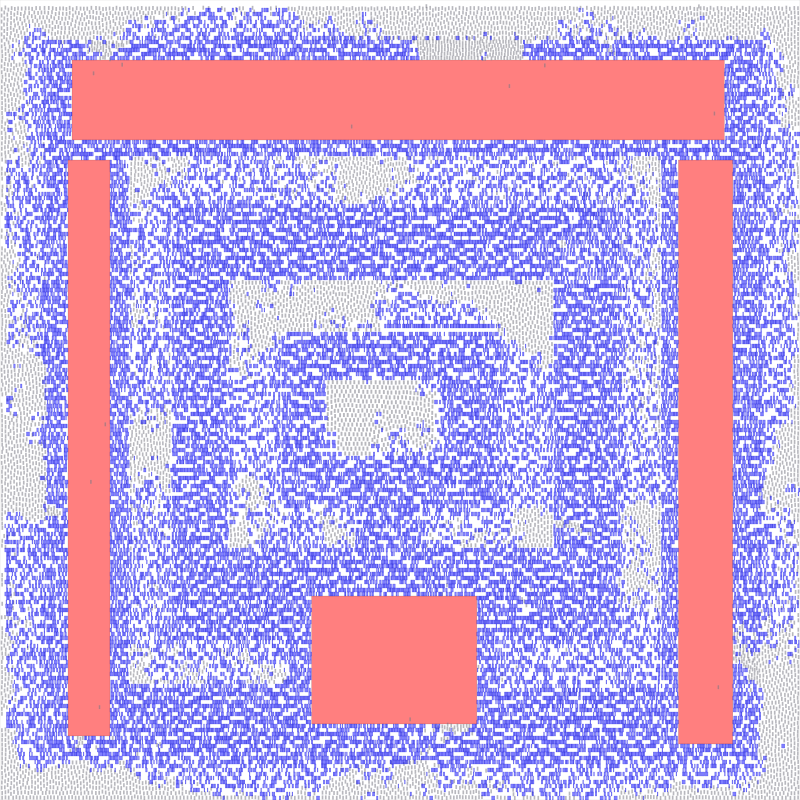}}
    \subfloat[pci\_a (non-WM)]{\label{f:design4} \includegraphics[width=0.2\linewidth]{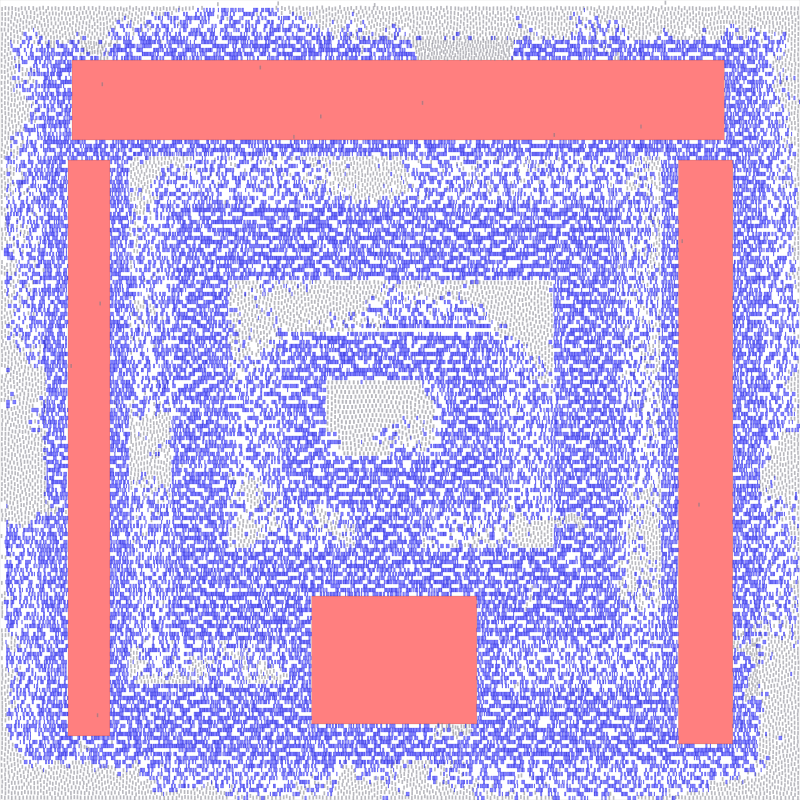}} 
    \subfloat[perf\_1 (WM)]{\label{f:design1} \includegraphics[width=0.2\linewidth]{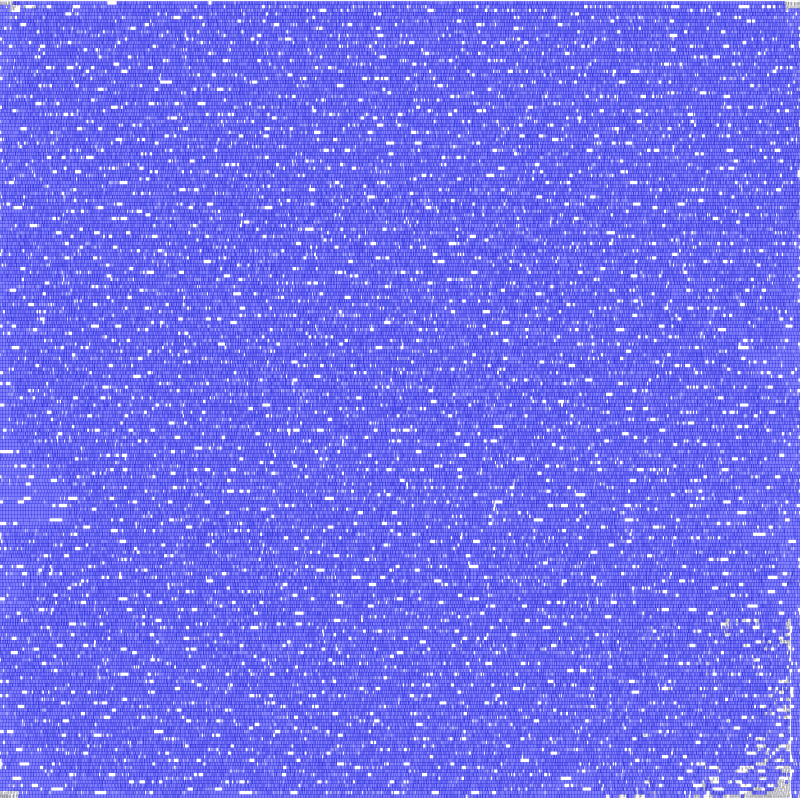}}\\
    \subfloat[perf\_1 (non-WM)]{\label{f:design2} \includegraphics[width=0.2\linewidth]{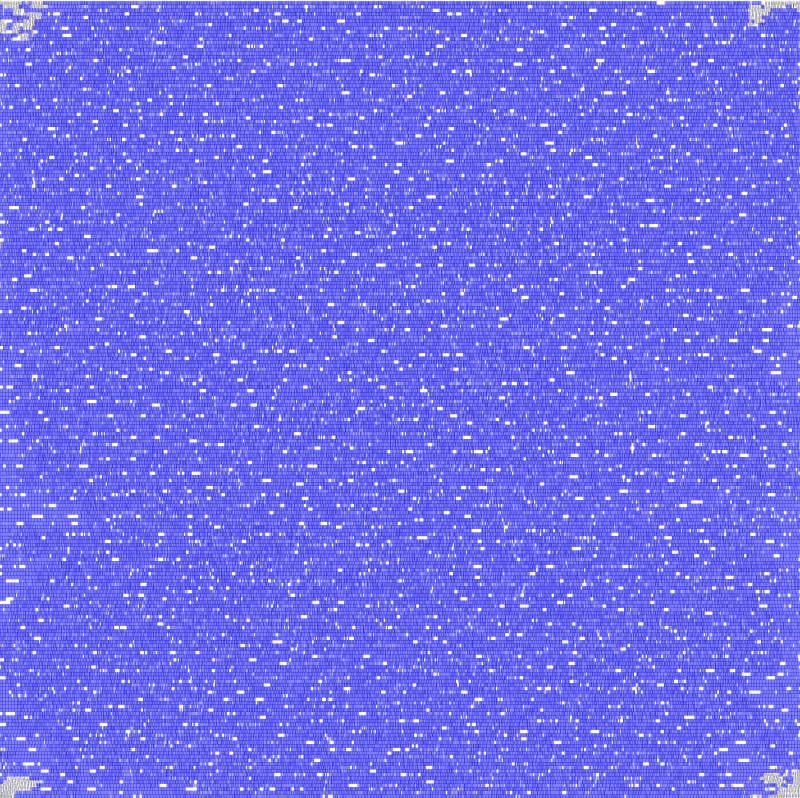}} 
    \subfloat[ispd19test4 (WM)]{\label{f:design5} \includegraphics[width=0.2\linewidth]{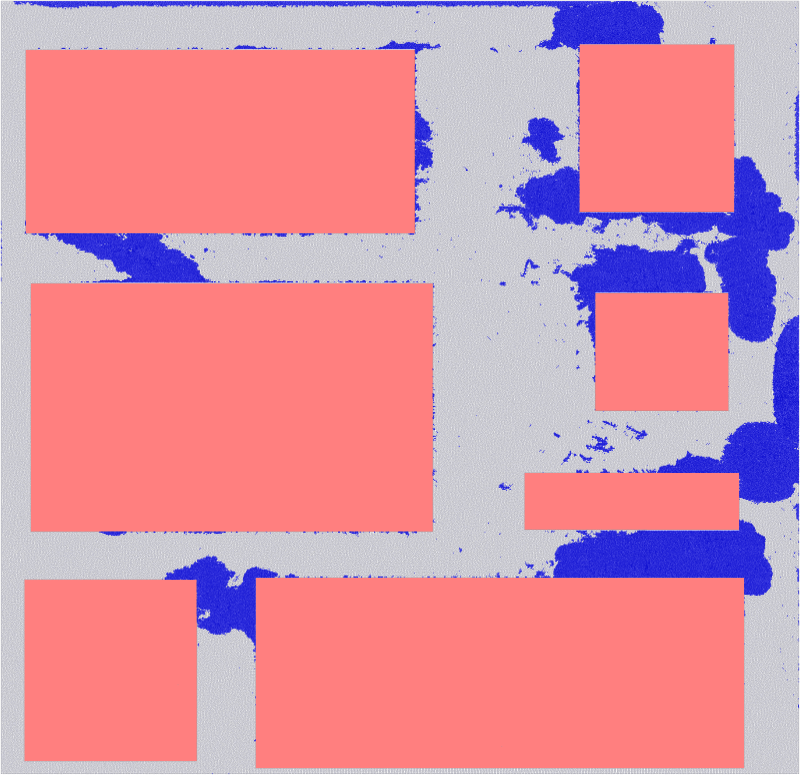}} 
    \subfloat[ispd19test4 (non-WM)]{\label{f:design6} \includegraphics[width=0.2\linewidth]{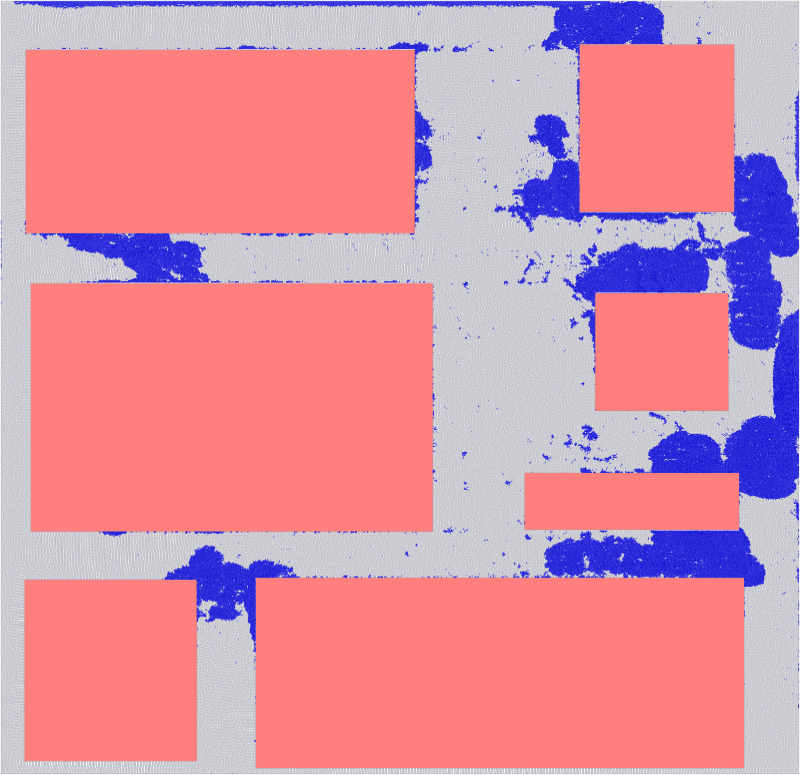}}
    \subfloat[superblue7 (WM)]{\label{f:design9} \includegraphics[width=0.2\linewidth]{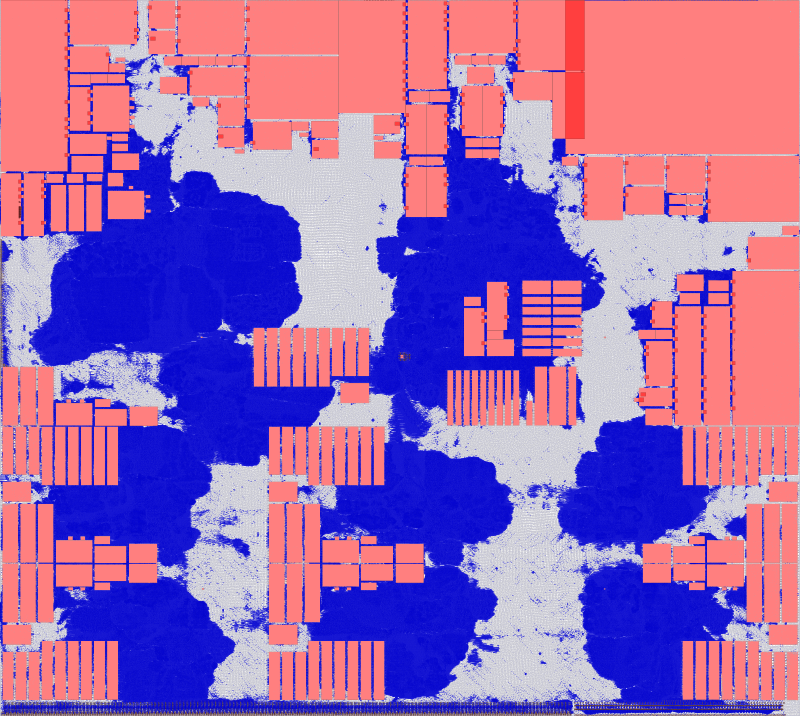}}
    \subfloat[superblue7 (non-WM)]{\label{f:design9} \includegraphics[width=0.2\linewidth]{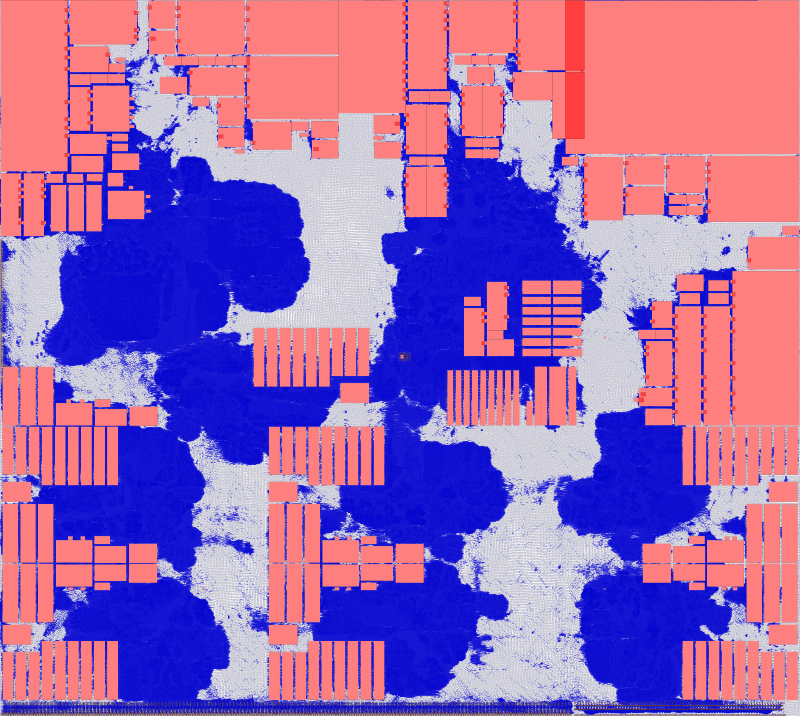}}
    \caption{Watermarked Design Examples. The \textcolor{blue}{blue} cells are the standard cells, and the \textcolor{red}{red} cells are the macros. We display watermark examples without design constraints in Figure~\ref{f:design1}-~\ref{f:design2}, with fence regions and macros in Figure~\ref{f:design3}-~\ref{f:design4} and with macros in Figure~\ref{f:design5}-~\ref{f:design9}.}
    \label{fig:example}
\end{figure*}
%\subfloat[superblue19]{\label{f:design7} \includegraphics[width=0.4\linewidth]{figs/superblue19.png}}

\subsection{Additional Attack Results on Timing-driven Placer} \label{sec:addition_attack}

We include the additional plots for timing-driven placer attacks in Figure~\ref{fig:timing_attack_results}.

\begin{figure*}[!ht]
    \centering
    \subfloat[Swap location attack (0.1\%)]{\label{f:append_sla_10_attack} \includegraphics[width=0.25\linewidth]{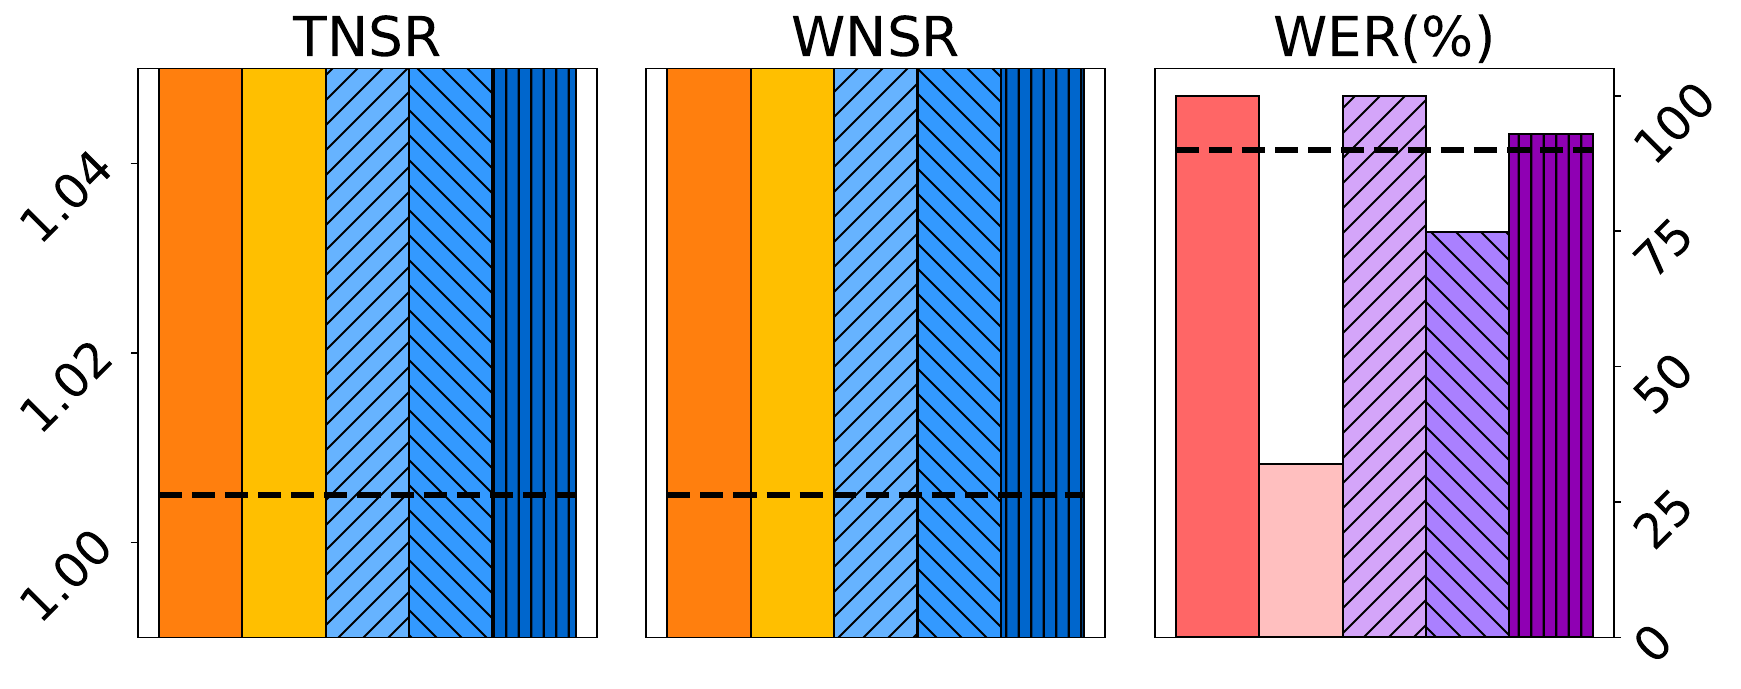}}
    \subfloat[Swap location attack (0.5\%)]{\label{f:append_sla_50_attack} \includegraphics[width=0.25\linewidth]{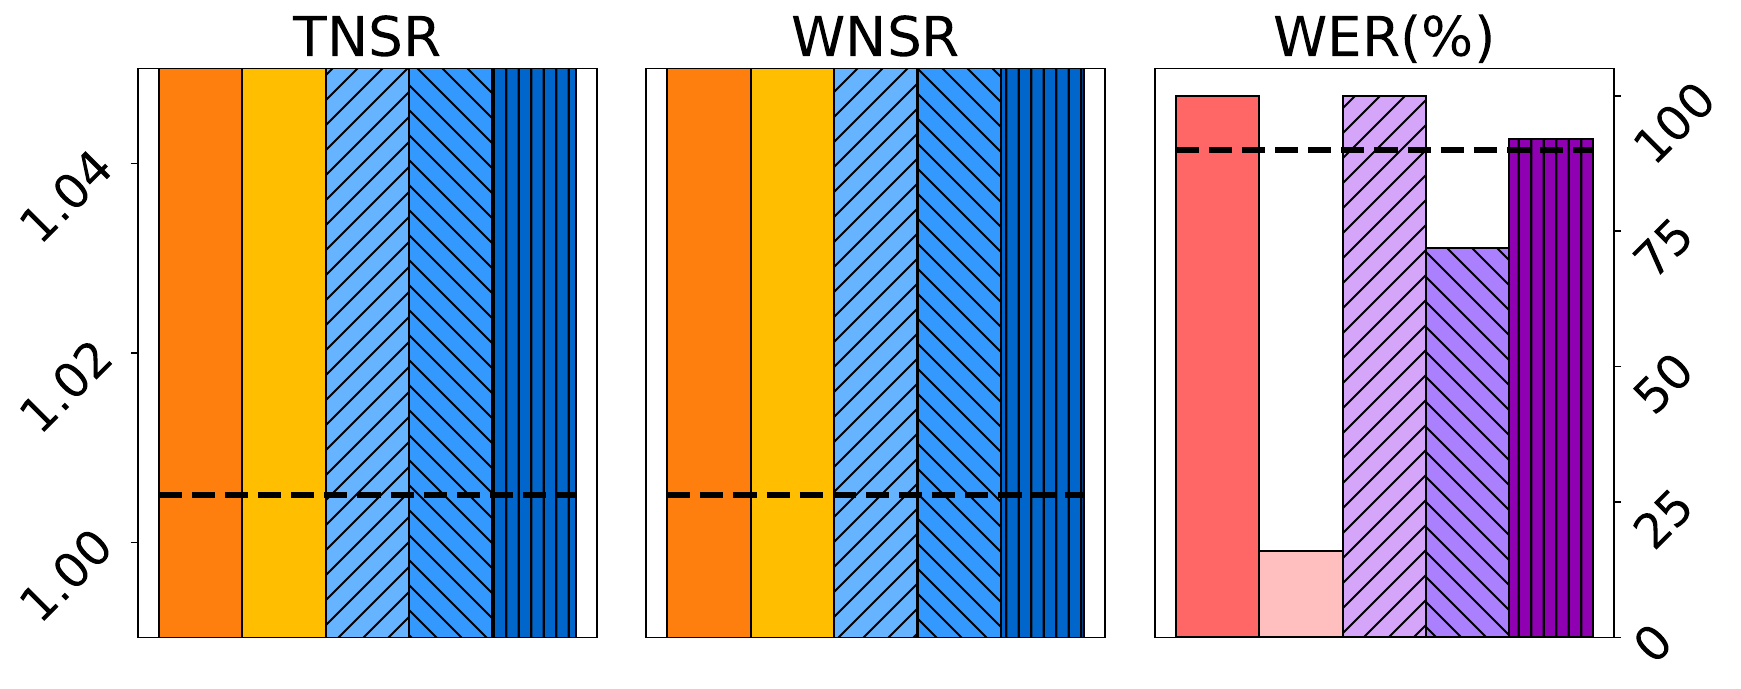}} 
    \subfloat[Constraint perturbation attack (0.1\%)  ]{\label{f:append_cpa_0.001} \includegraphics[width=0.25\linewidth]{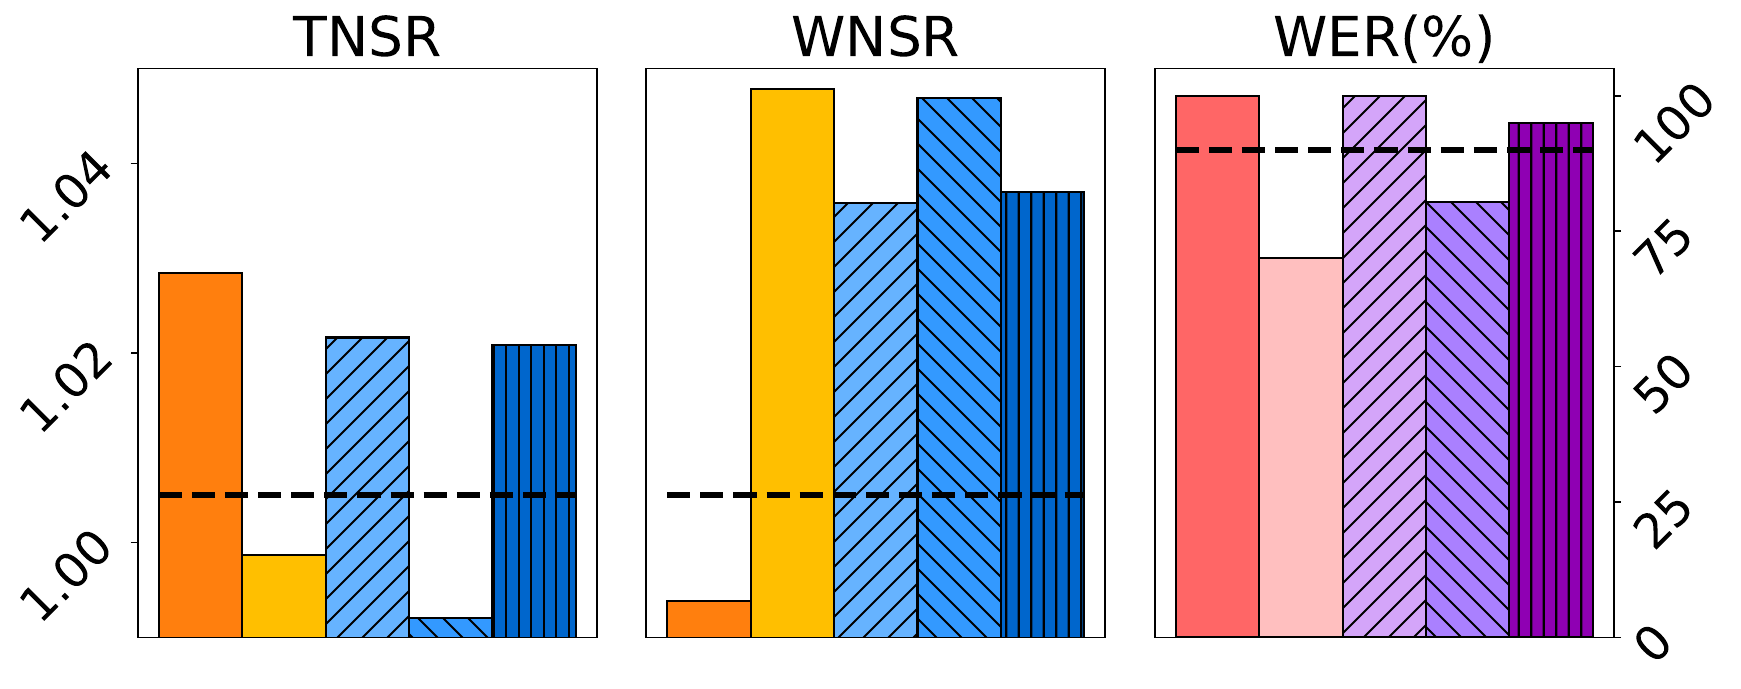}} 
    \subfloat[Constraint perturbation attack (1\%) ]{\label{f:append_cpa_0.01} \includegraphics[width=0.25\linewidth]{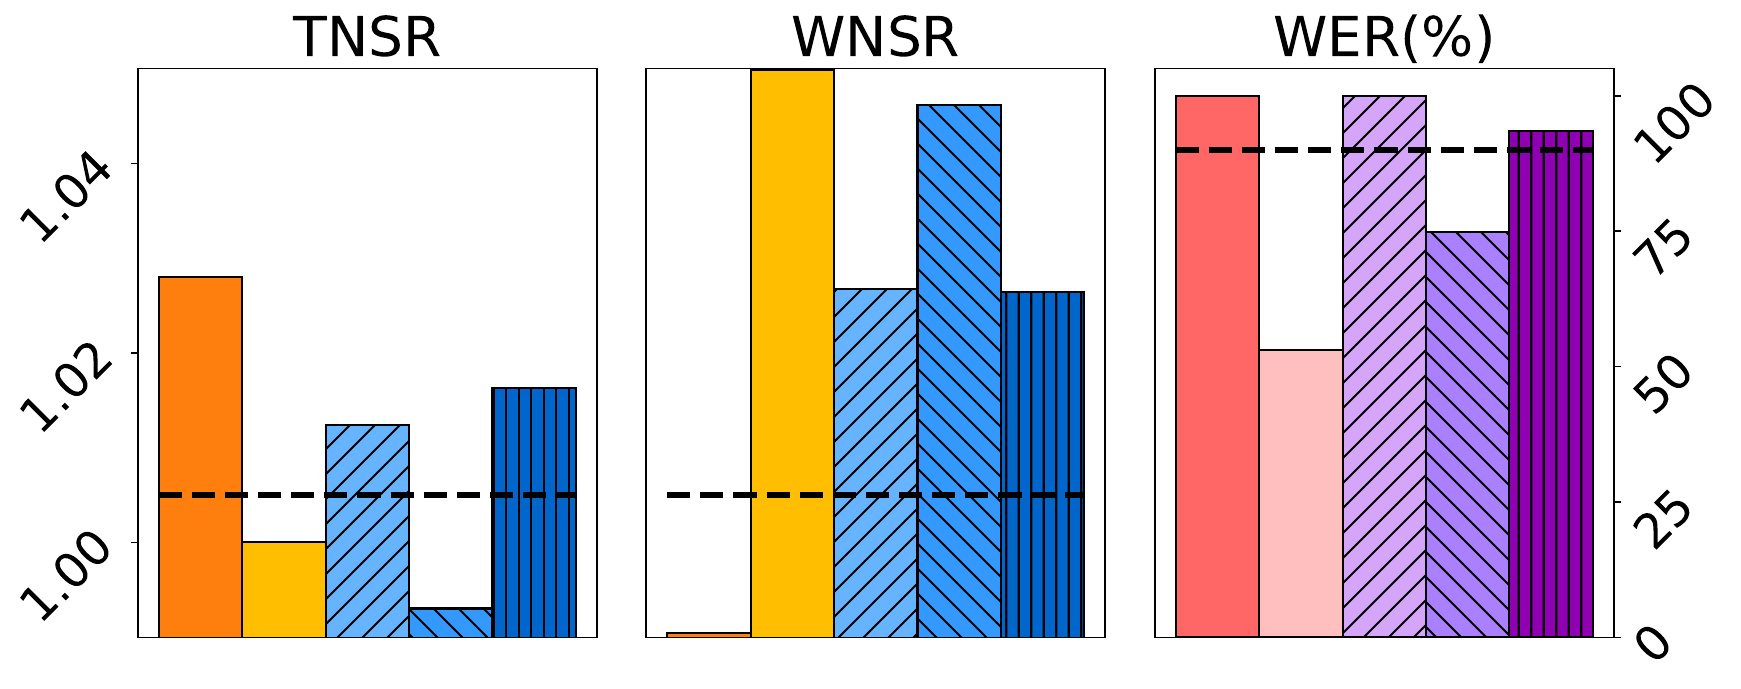}} \\
    \subfloat[Constraint perturbation attack (10\%)]{\label{f:append_cpa_0.1} \includegraphics[width=0.25\linewidth]{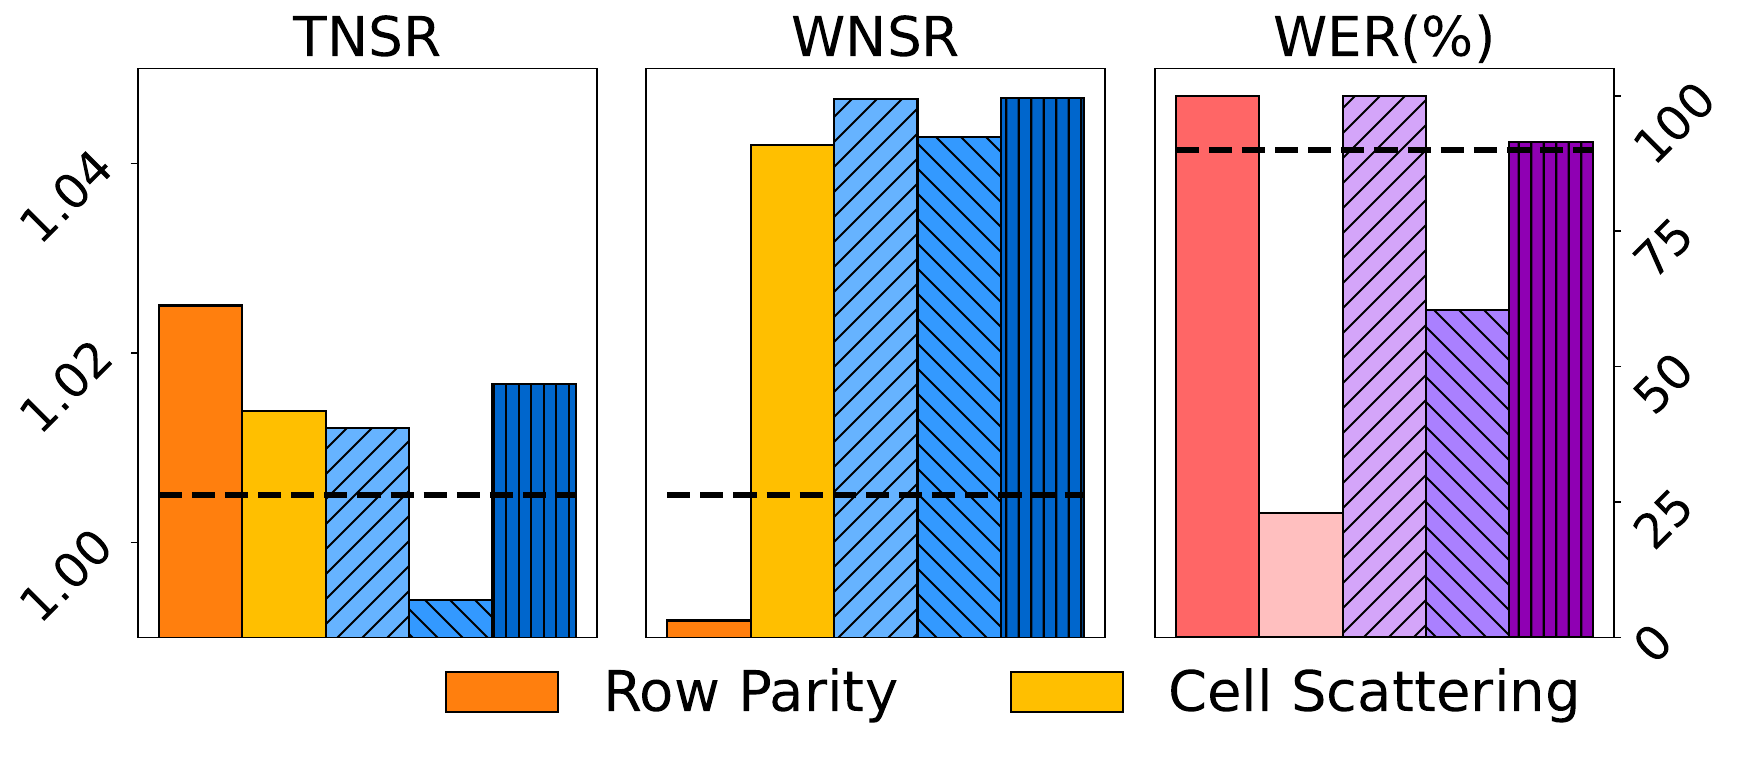}} 
    \subfloat[Optimization attack ]{\label{f:append_eco_attack} 
    \includegraphics[width=0.25\linewidth]{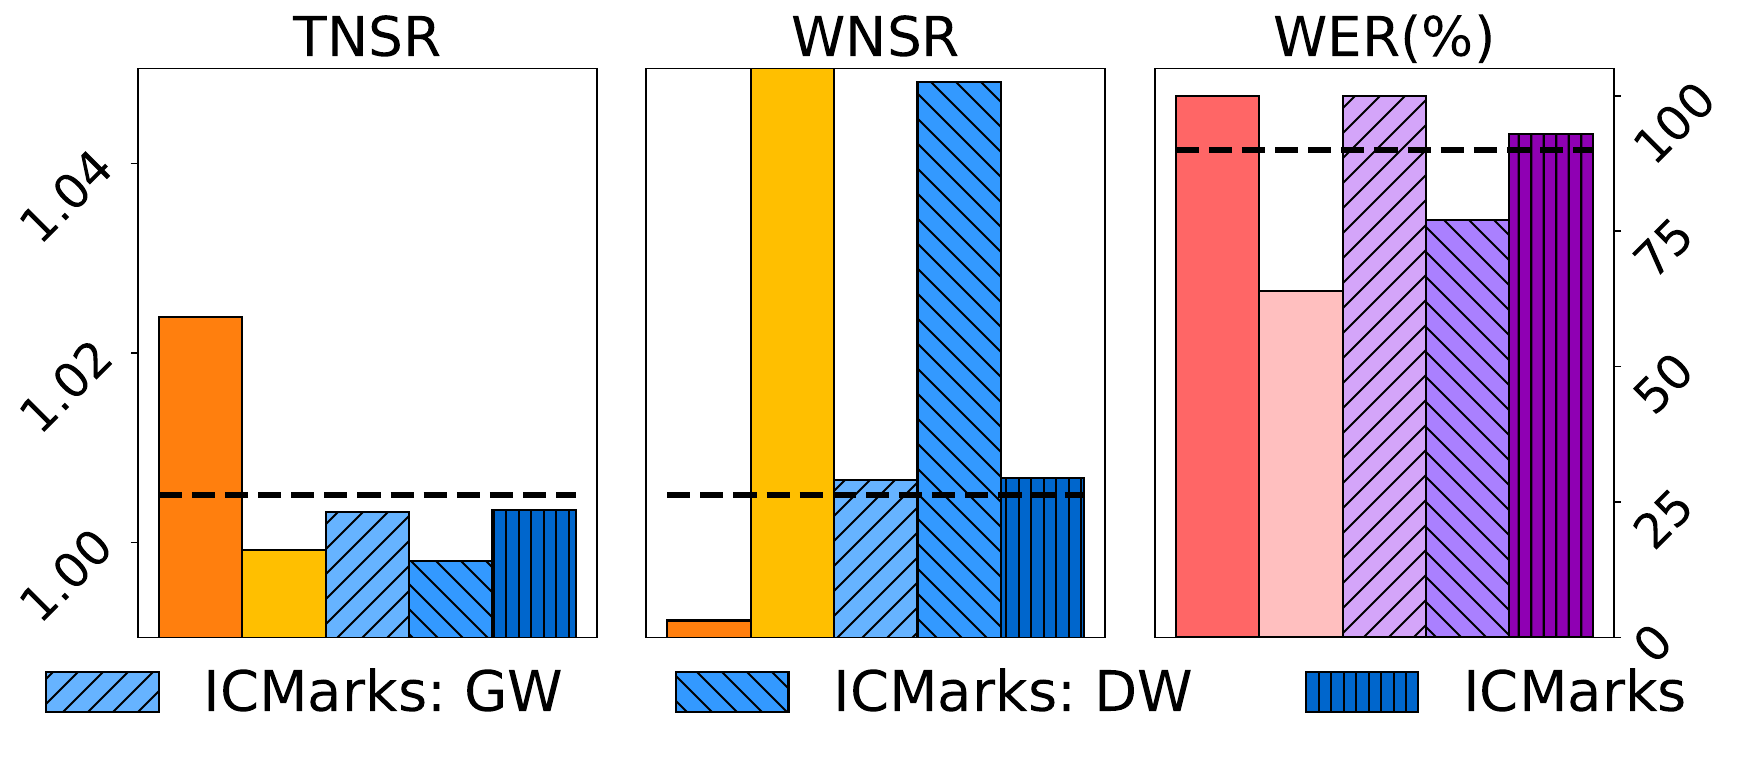}}   
    \subfloat[Adaptive region attack (top-1) ]{\label{f:append_ada_attack} \includegraphics[width=0.25\linewidth]{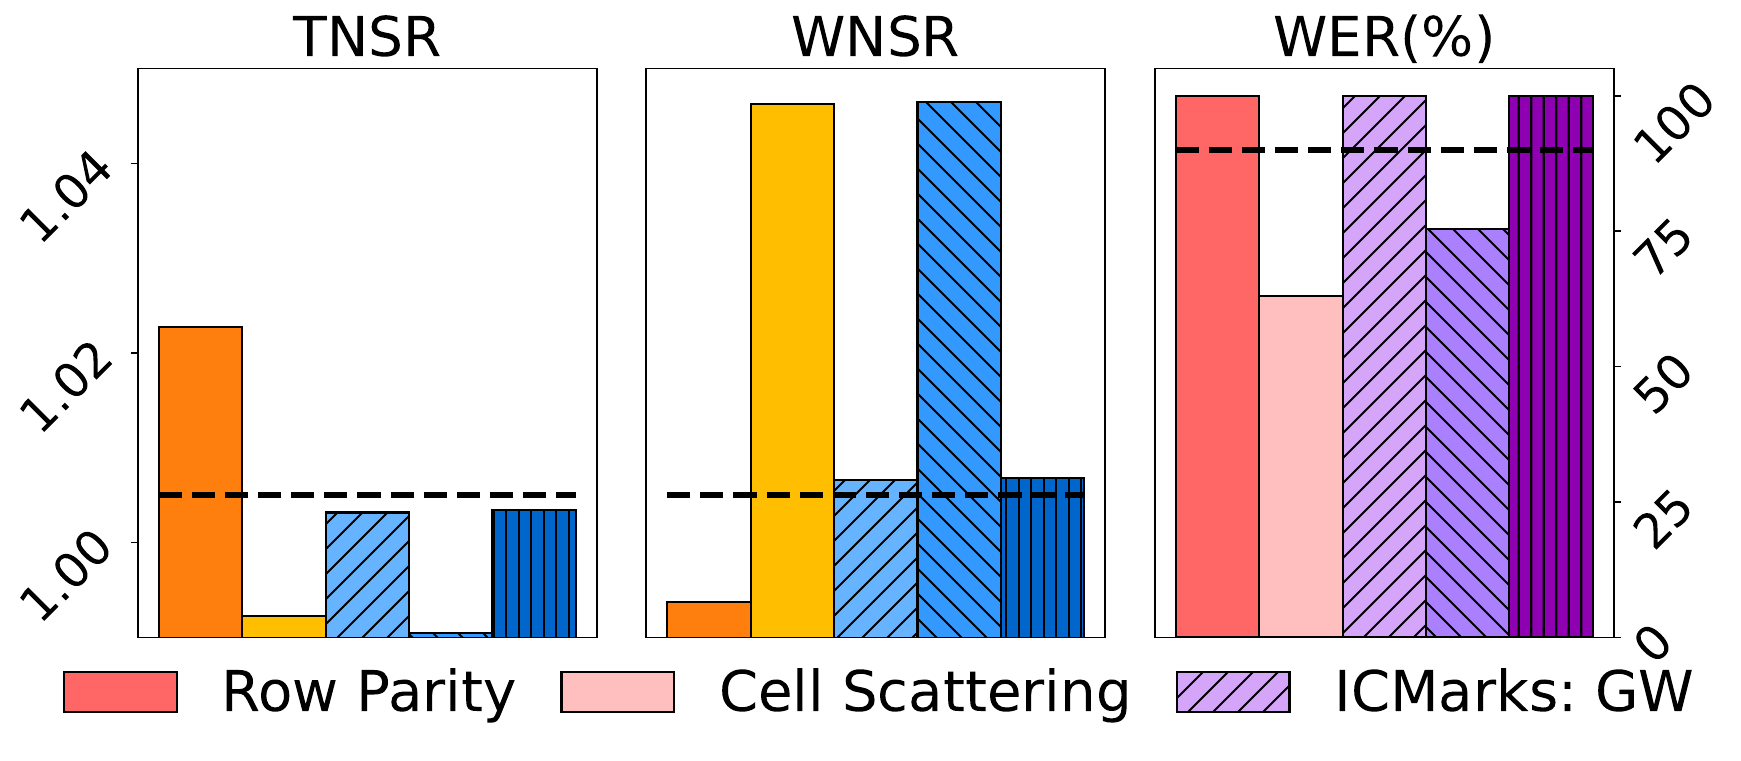}}
   \subfloat[Adaptive region attack (top-5)]{\label{f:ada_attack} \includegraphics[width=0.25\linewidth]{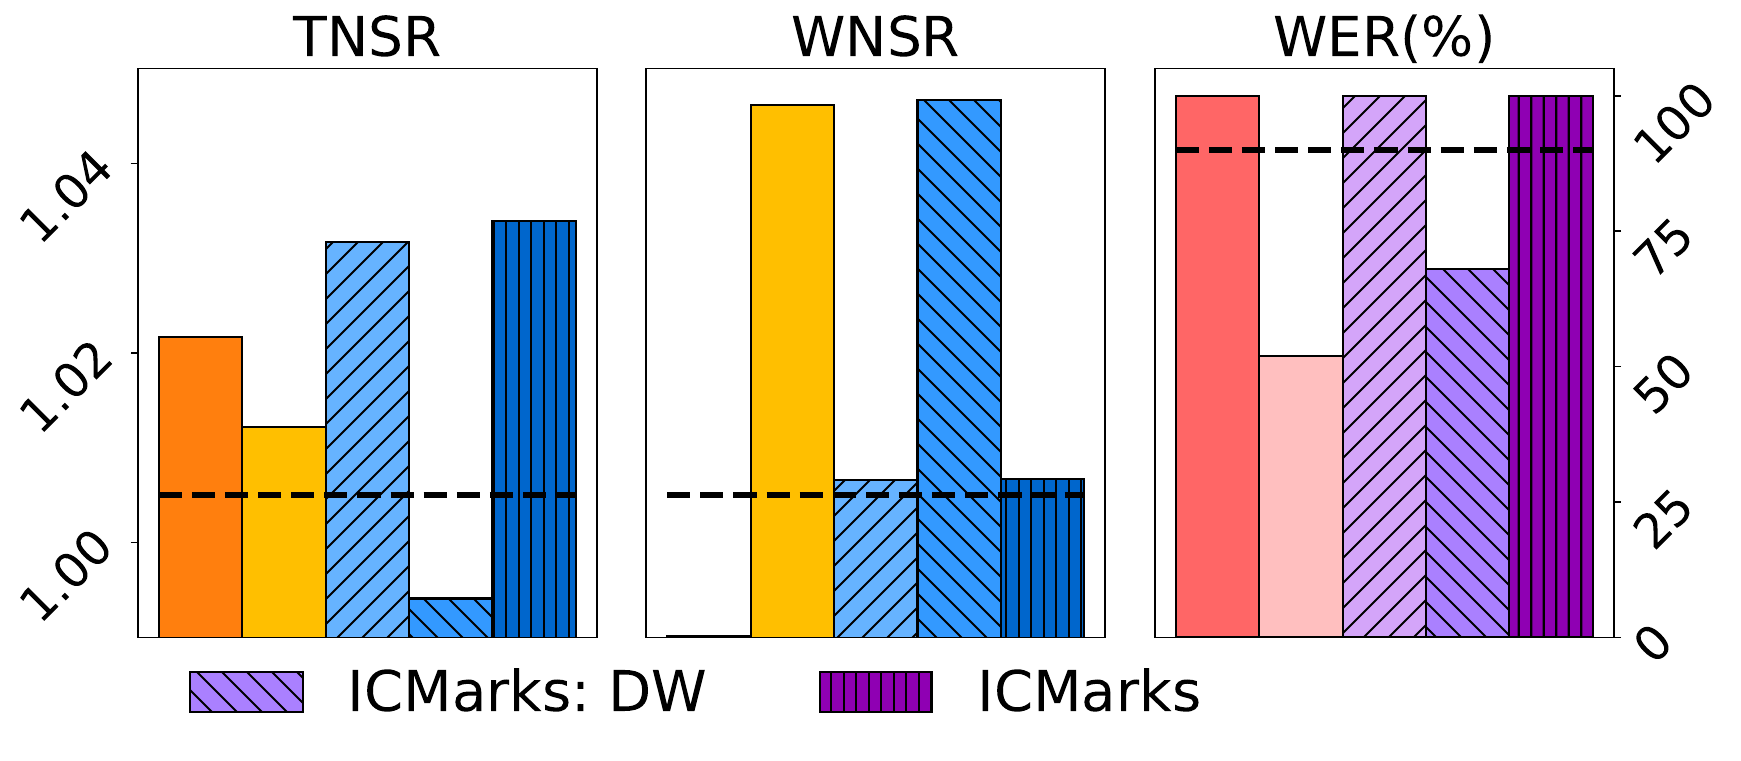}}
    \caption{Watermarking performance under different attacks for Timing Driven Placer on ICCAD'2015 benchmarks~\cite{7372671}. The black dotted line in the two left subfigures denotes the quality degradation threshold as 1.005, and the black dotted line in the rightmost subfigure denotes the watermark extraction threshold as 90\%.}
 
    \label{fig:timing_attack_results}
\end{figure*}



%\section{Additional Experiments }
%\paragraph{Experiment Setup}
%\sys{} is implemented with Python 3.9 and benchmarked on a Linux Ubuntu system equipped with four NVIDIA TITAN Xp GPUs, each with 12 GB RAM, and 48 Intel(R) Xeon(R) CPUs, accompanied by 128 GB RAM.
%The watermarking methodology of \sys{} can be integrated into any VLSI physical design framework, and we chose to build upon the open-source placement framework, DREAMPlace~\cite{lin2019dreamplace} and the open-source routing framework CUGR~\cite{9218646}, to demonstrate its viability. We use DREAMPlace 4.0~\cite{9774725} to perform placement algorithms on timing-driven datasets. The timing metrics are measured by OpenTimer~\cite{huang2020opentimer}. The DREAMPlace family~\cite{lin2019dreamplace, 9774725} accelerates the state-of-the-art placement algorithm ePlace~\cite{lu2015eplace}/RePlAce~\cite{cheng2018replace} on a GPU and maintain the same level of performance. 



%\paragraph{Dataset Statistics and Parameter Settings}
%The detailed dataset statistics for ISPD'2005, ISPD'2015, ISPD'2019, and ICCAD'2015 are summarized as Table~\ref{tab:dataset_statistic}. In GW and \sys, our sliding window's size and stride are the factor of row height of the design. 
%Depending on the size of the designs and the distributions of the cells. This is pre-defined by the designer. 
%As for the scoring hyperparameters, we set the default values of $\alpha$ = 0.1, $\beta$ = 0.1, and $\gamma$ = 1.  If the default values of the hyperparameters results in more than $5\%$ wirelength degradation, we perform a grid search for $\alpha$ = \{0, 0.1, 0.5\} and $\beta$=\{0, 0.1, 0.5\} and report the best-performing hyperparameters. 
%Table~\ref{tab:dataset_statistic}. 
%In the \textit{Detailed Watermarking} phase, $d_x$ is set to one unit, and $d_y$ is set to 1-row height.




 



%In this subsection, we provide additional experiment results for timing-driven placement watermarking performance under various attacks as proposed in Section~\ref{sec:removal_attack}.


    \begin{comment}


\paragraph{Comparison with routing-based watermarking} ~\label{sec:routing_wm_append}
Extensive experiments in the previous sections demonstrated \sys{} incurs no routed wirelength degradations to the layouts. Nevertheless, in this subsection, we compare \sys{} with the routing-based watermarking approach~\cite{1510323} in Figure~\ref{fig:routing_wm_compare} on ISPD'2019~\cite{liu2019ispd}. The routing-based watermarking bends wires and introduces a constant 4 unit wirelength into the layout per signature bit insertion. 
All inserted watermarks are successfully extracted, and we skip this metric in the figure.  From here, we can find for small signature insertions, \sys{} gets much better RWLR compared with routing-based watermarking baselines. Because no additional RWLR overhead is introduced by \sys{}. However, the small signature insertion of \sys{} does not yield weak watermark protections as reflected by the p-value $P_c$ in Table~\ref{tab:security}. 

\begin{figure}[!ht]
    \centering
    \includegraphics[width= 0.7\columnwidth]{figs/capacity_routing.pdf}
     \caption{Routed WireLength Rate (RWLR) degradations compared with routing-based watermarking. }%\textcolor{red}{extend to 100k and 200k. like 5\% of the cells(see what's happen for specific layout.change different marker for two sets.=)}
     \vspace{-0.5cm}
    \label{fig:routing_wm_compare}
\end{figure}


\paragraph{Timing-driven Placer Routed Performance} We also report the routed wirelength for timing-driven placer in Table~\ref{tab:iccad2015_wl}. From here, we can find apart from timing metrics and the estimated wirelength from PWLR, \sys{} maintains good routed wirelength performance compared with baseline Row Parity in the watermarked layout. The average routed wirelength of \sys{} is reduced by XX\% compared with the Row Parity baseline.

\begin{table}[!h]
\resizebox{\columnwidth}{!}{%
\begin{tabular}{|c|c|c|c|c|}
\hline
Design & Row Parity & \sys: GW & \sys: DW & \sys \\ \hline
superblue1 &  & &  & \\ \hline
superblue3 &  & &  & \\ \hline
superblue4 &  & &  & \\ \hline
superblue5 &  & &  & \\ \hline
superblue7 &  & &  & \\ \hline
superblue10 &  & &  & \\ \hline
superblue16 &  & &  & \\ \hline
superblue18 &  & &  & \\ \hline
W-Avg &  & &  & \\ \hline
\end{tabular}%
}
\caption{ICCAD'2015~\cite{7372671} timing-driven routed wirelength.}
\label{tab:iccad2015_wl}
\end{table}
\end{comment}
\begin{comment}
    

\paragraph{Timing-driven Placer Watermark Overhead}~\label{sec:overhead_timing_append}
The watermark overhead is summarized in Table~\ref{tab:iccad2015_overhead}. It indicates that akin to nonlinear placement scenarios, both Row Parity and \sys: DW introduces negligible watermark overhead during the insertion process. In contrast, \sys: GW and \sys{} incur an average watermarking overhead of 14 minutes and 15 minutes, respectively. This increased overhead is attributable to the execution of timing analysis every 1k iterations; a prolonged convergence iteration subsequently leads to more timing analyses. It is worth noting that timing analysis emerges as the primary contributor to this additional overhead. Nonetheless, these overhead durations are deemed justifiable, especially when considering the average reductions in TNSR by 6.16\%, WNSR by 2.57\%, and WLR by 0.2\% in comparison to the baseline Row Parity.
% Please add the following required packages to your document preamble:
% \usepackage{graphicx}
\begin{table}[!h]
\resizebox{\columnwidth}{!}{%
\begin{tabular}{|c|c|c|c|c|}
\hline
Design & Row Parity & \sys: GW & \sys: DW & \sys \\ \hline
superblue1 & \textbf{35.21} & 900.38 & 91.08 & 993.72 \\ \hline
superblue3 & \textbf{7.01} & 618.68 & 39.73 & 665.04 \\ \hline
superblue4 & \textbf{6.02} & 529.43 & 26.57 & 618.14 \\ \hline
superblue5 & \textbf{21.00} & 697.97 & 48.88 & 785.68 \\ \hline
superblue7 & \textbf{8.37} & 1123.14 & 127.32 & 1192.06 \\ \hline
superblue10 & \textbf{62.80} & 1463.15 & 221.22 & 1555.85 \\ \hline
superblue16 & \textbf{3.39} & 446.28 & 7.24 & 494.12 \\ \hline
superblue18 & 47.39 & 343.28 & \textbf{8.15} & 393.28 \\ \hline
W-Avg & \textbf{25.59} & 875.64 & 91.97 & 949.90 \\ \hline
\end{tabular}%
}
\caption{ICCAD'2015~\cite{7372671} timing-driven placement watermarking overhead (s).}
\label{tab:iccad2015_overhead}
\end{table}
\end{comment}

%\paragraph{Timing-driven Placement Watermark Removal Attacks}~\label{sec:attack_timing_append}
%We include the additional attack performance of the timing-driven placement watermarking in Figure~\ref{fig:timing_attack_results}. We perform similar attack settings as Section~\ref{sec:removal_attack} on ICCAD 2015 datasets. 
%We find \sys{} achieves robustness and the watermarks are highly extractable under all the attacks. Row Parity becomes more resilient when the layout size becomes larger, but \sys{} and its submodule \sys:GW achieve comparable WER performance and can accommodate more signatures without degrading the timing-driven layout quality.  
 

 
%\paragraph{Watermarking Overhead} 
%From Table~\ref{tab:watermark_overhead}, we report the additional time it takes to insert the watermark. 
%It reveals that the computational overhead improvements for \sys: DW and Row Parity, when contrasted with non-watermarking layouts, remain below 5 seconds. The marginal overhead introduced by both methods are reasonably negligible. Conversely, for \sys: GW and \sys{}, introducing an auxiliary watermarked region and cells as a co-optimization criterion takes more iterations for the placement algorithm to converge. Consequently, the overhead associated with watermark insertion becomes longer. However, when considering the quality enhancements—0.02\% PWLR and 0.45\% RWLR for \sys: GW, and 0.32\% PWLR and 0.44\% RWLR for \sys—compared to even non-watermarked layouts, the additional average watermark overheads of 43 seconds for \sys: GW and 52 seconds for \sys{} emerge as justifiable.

%\begin{table}[!h]
%\resizebox{\columnwidth}{!}{%
%\begin{tabular}{|c|c|c|c|c|}
%\hline
%Design & Row Parity & \sys: GW & \sys: DW & \sys \\ \hline
%ISPD'2005& 1.90 & 36.01 & 2.41 & 40.66 \\ \hline
%ISPD'2015 & 0.38 & 7.92& 0.58 & 9.95 \\ \hline
%ISPD'2019 &  1.05 &17.06 &0.53 &16.09  \\ \hline
%\end{tabular}%
%}
%\caption{Watermarking Overhead (in seconds) for different benchmarks}
%\label{tab:watermark_overhead}
%\end{table}
%\section{Additional Related Work}
%%\label{sec:related}
%\input{files/6_related}
